# Supplementary material for: TLDR: Text Based Last-layer Retraining for Debiasing Image Classifiers
Source: arXiv:2311.18291 source file (2024-12-07)
Supplement: Supplementary file 1 [file Supp_spu_filter.tex]

As stated in Section \ref{sec:filter}, we also try filtering $\mathcal{T}^a$ by comparing the averaged logits given by $h_\phi$ when the $t_j^a$ is present or absent.
That is, we compare $\mathbb{E}_i[\mathbb{P}(h_\phi(\Pi(\bm z^{\text{CLIP}}_{P_1(t^y_i)})) = y)]$ and $\mathbb{E}_i[\mathbb{P}(h_\phi(\Pi(\frac{\bm z^{\text{CLIP}}_{P_1(t^y_i)} + \bm z^{\text{CLIP}}_{P_1(t^a_j)}}{2})) = y)]$ for each $t^a_j$ where $t^y_i \in \mathcal{T}^y_{\text{filter}}$.
To measure the significance of the difference in means, we adopt the paired t-test.
Since the statistical test is performed on all $t^a_j \in \mathcal{T}^a_{\text{filter}}$, we need to correct the p-value of each $t^a_j$ to control the False Discovery Rate (FDR).
Therefore, we perform the Benjamini-Hochberg \cite{FDR} procedure to correct the p-values to control the FDR to be less than 0.05.
Based on this procedure, we can effectively filter $t_j^a$ which significantly affects the prediction of $h_\phi$ without introducing an additional hyperparameter.

The experimental result with the t-test based filtering is shown in the last row of Table \ref{tab:t_test}.
The effect of the t-test filter seems to be marginal.
We conjecture that the semantic filter is sufficient for $\mathcal{T}^a$.
% filtering words which affects the prediction of $h_\phi$ significantly.
To validate this conjecture, we replace the semantic filter for $\mathcal{T}^a$ with the t-test based filter and the results are shown in the second row of the Table \ref{tab:t_test}.
Indeed, the semantic filter and the t-test based filter seem to have an equivalent effect on the performance.
Hence, we use the semantic filter instead of the t-test based filter in our method because of its simplicity.

% We compare the mean logit when the text contains words about the spurious attributes and when it does not.
% That is, we compare $\mathbb{E} \mathbb{P}[\hat{y}| Pz^{\text{CLIP}}_{\text{text}_y}]$ and $\mathbb{E} \mathbb{P}[\hat{y}|P\frac{z^{\text{CLIP}}_{\text{text}_{y_i}} + z^{\text{CLIP}}_{\text{text}_{a}}}{2}]$, with expectation with respect to filtered class name synonyms.
% We evaluate the significance of the difference of mean using the paired t-test.
% Furthermore, as we perform the statistical test for every word generated for \textit{spurious attributes names}, correction of the p-value is needed to control the false discovery rate (FDR).
% Therefore, we perform the Benjamini-Hochberg procedure to correct the p-value to control the FDR to be less than 0.05.
% Based on this procedure, we can effectively filter the words that significantly affect the prediction of the trained linear classifier without introducing an additional hyperparameter.
